# Supplementary material for: Porous mechanical metamaterials as interacting elastic charges
Source: arXiv:1709.00328 ancillary file (2017-08-29)
Supplement: Supplementary file 1 [file SI.pdf]

# Supplemental Material for
# *Porous mechanical metamaterials as interacting elastic charges*

Gabriele Librandi,[1,*] Michael Moshe,[2,3,*] Yoav Lahini,[1,4] and Katia Bertoldi[1,5,†]

[1]*Harvard John A. Paulson School of Engineering and Applied Sciences, Harvard University, Cambridge, Massachusetts 02138, USA*
[2]*Physics Department, Harvard University, Cambridge Massachusetts , USA*
[3]*Department of physics, Soft matter program, Syracuse University, New-York , USA*
[4]*Raymond and Beverly Sackler School of Physics and Astronomy, Tel Aviv University, Ramat Aviv, Tel Aviv 69978, Israel*
[5]*Kavli Institute, Harvard University, Cambridge, MA 02138*

## EXPERIMENTS

The three samples tested for this study were fabricated out of polyurethane foam sheets (PORON 4701-40 Soft from Rogers Corporation) with thickness $t = 12.7$ mm. All holes were introduced into the foam sheets using a CO2 laser system (VersaLaser 3.50, Universal Laser Systems) with the following settings: Power 100 % and Speed 10 % (all other laser parameters were left as default). Note that four runs were required for the laser to cut completely through the thickness of the sheets. Finally, the samples were sprayed with white painting to facilitate postprocessing via digital image analysis.

*Sample #1* has size 89.5×89.5 mm and comprises a 8×8 square array of circular holes with radius $r_0 = 4.1842$ mm and center-to-center distance $d = 10$ mm, resulting in an initial porosity $\Psi = \pi r_0^2/d^2 = 0.55$.

*Sample #2* has size 155×149.5 *mm* and comprises a 10×11 triangular array of circular holes with radius $r_0 = 6.4945$. The holes are located on the vertices of an equilateral triangle which edge $d = 15$ mm, resulting in an initial porosity $\Psi = \pi r_0^2/(d^2 \cos\pi/3) = 0.68$.

*Sample #3* has size 89×154 mm and comprises a 8×8 rectangular array of elliptical holes with major and minor semi-axis $a = 7.5606$ mm and $b = 3.9828$ mm and center-to-center distance $d_x = 17.2$ mm and $d_y = 10$ mm, resulting in an initial porosity $\Psi = \pi a\, b/(d_x d_y) = 0.55$.

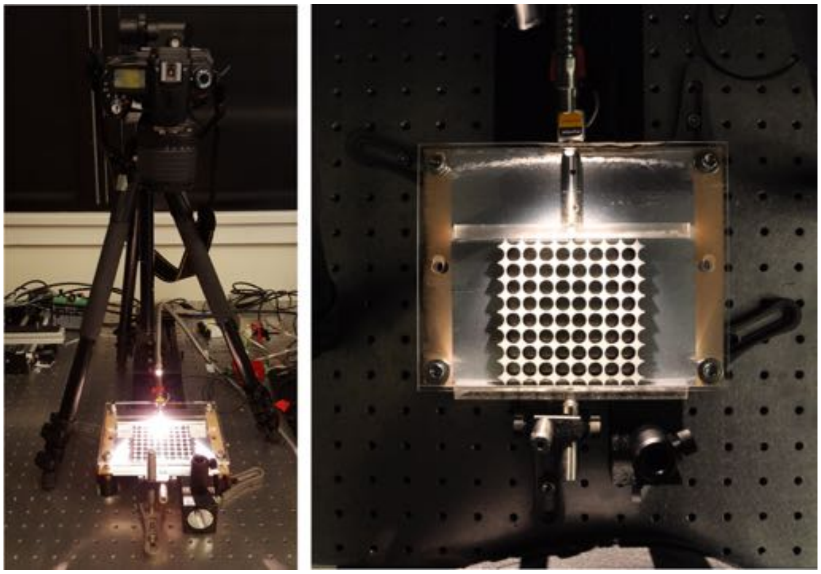

FIG. S1. Experimental setup

All specimens were tested with a built-in-house uniaxial loading machine at the rate of 0.5 mm/sec. The apparatus consists of a Thorlabs breadboard and a Thorlabs long travel stage controlled through a Matlab code and is equipped with a 0.044 N load cell, see Fig. S1. During the uniaxial compression tests, videos were recorded using a digital camera (Nikon D90 SLR), focusing on the four central holes (see Fig. S2(a)) to both reduce boundary effects and to achieve higher resolution. The captured videos were then analyzed by digital image processing (Matlab).

## COMPARING EXPERIMENTS TO THEORY

We verify the capability of elastic charges to capture the changes in hole shape and orientation triggered by the applied deformation in porous mechanical metamaterials by comparing the experimentally observed deformation patterns to those predicted by our theory. To make such comparison, we extract from the captured videos the experimental displacement field of the hole boundaries. To this end, we first track the boundaries of the holes at different levels of applied deformation using the software Matlab (see red lines in Fig. S2 (a) and (b)) and extract the $x$ and $y$ coordinates (with respect the centroid of each hole) of each point on the boundary. Note that, to facilitate the subsequent fitting procedure, the profile of the extracted boundaries is smoothed by defining a spline passing through these points (see dotted lines in Fig. S2 (c)-(f)). Having checked that the change in perimeter of each hole is negligible during the tests, we then reconstruct the displacement field for each point on the boundary by

tracking a single marker placed next to each hole (see red circular marker in Fig. S2 (a) and (b)). In fact, because of the perimeter conservation, the displacement of a point $P$ located at a distance $s$ from such marker can be simply calculated as

$$\begin{aligned} u_r(s) &= (x(s) - x_0(s))\cos\theta \ + (y(s) - y_0(s))\sin\theta, \\ u_\theta(s) &= -(x(s) - x_0(s))\sin\theta + (y(s) - y_0(s))\cos\theta, \end{aligned} \tag{S1}$$

where $(x_0(s),\, y_0(s))$ and $(x(s),\, y(s))$ denote the coordinates of point $P$ in the undeformed and deformed configuration, respectively, and $\theta = \arctan{(y_0(s)/x_0(s))}$.

Having obtain the experimental displacement field of the hole boundary, we then determine the combination of the five charge parameters $p$, $q$, $h$, $\theta_q$ and $\theta_h$ that results in $u_r$ and $u_\theta$ (given by Eq. (7) in the main text) that best approximate the experimentally obtained ones. Finally, the deformed shape of the hole boundary as predicted by the elastic charges can be simply calculated as

$$\begin{aligned} x(s) &= x_0(s) + u_r\cos\theta - u_\theta\sin\theta, \\ y(s) &= y_0(s) + u_r\sin\theta \ + u_\theta\cos\theta. \end{aligned} \tag{S2}$$

where $u_r$ and $u_\theta$ are given by Eq. (7) in the main text evaluated for the optimal combination of parameters $p$, $q$, $h$, $\theta_q$ and $\theta_h$. As shown in Fig.S2 (d), (f) and (g) these coordinates describe the deformed configuration of the four central holes with high fidelity.

Finally, it is important to point out that that our approach requires comparison between points on the deformed configuration and their counterparts on the undeformed configuration. While this is easy to achieve in initially circular holes (since equally spaced points on a circle correspond to equally spaced angles), for holes with non circular shape (as the elliptical ones considered in this study) the tracking procedure is more delicate. To facilitate the tracking for the elliptical holes, we use the following procedure:

- *Step 1*: since an ellipse can be considered as an elongated circle, we identify the scaling factors that deform the ellipse into a circle with the same average radius. Then, we identify $N$ equally spaced points on the "virtual" circular configuration.
- *Step 2*: we rescale the deformed configuration with the same scaling factors, and consider the "virtual" deformed configuration as obtained from the "virtual" circular configuration through deformation.
- *Step 3*: being able to correctly compare points on the deformed configuration with their counterparts on the undeformed ones, we find the elastic charges resulting in the best fitting.

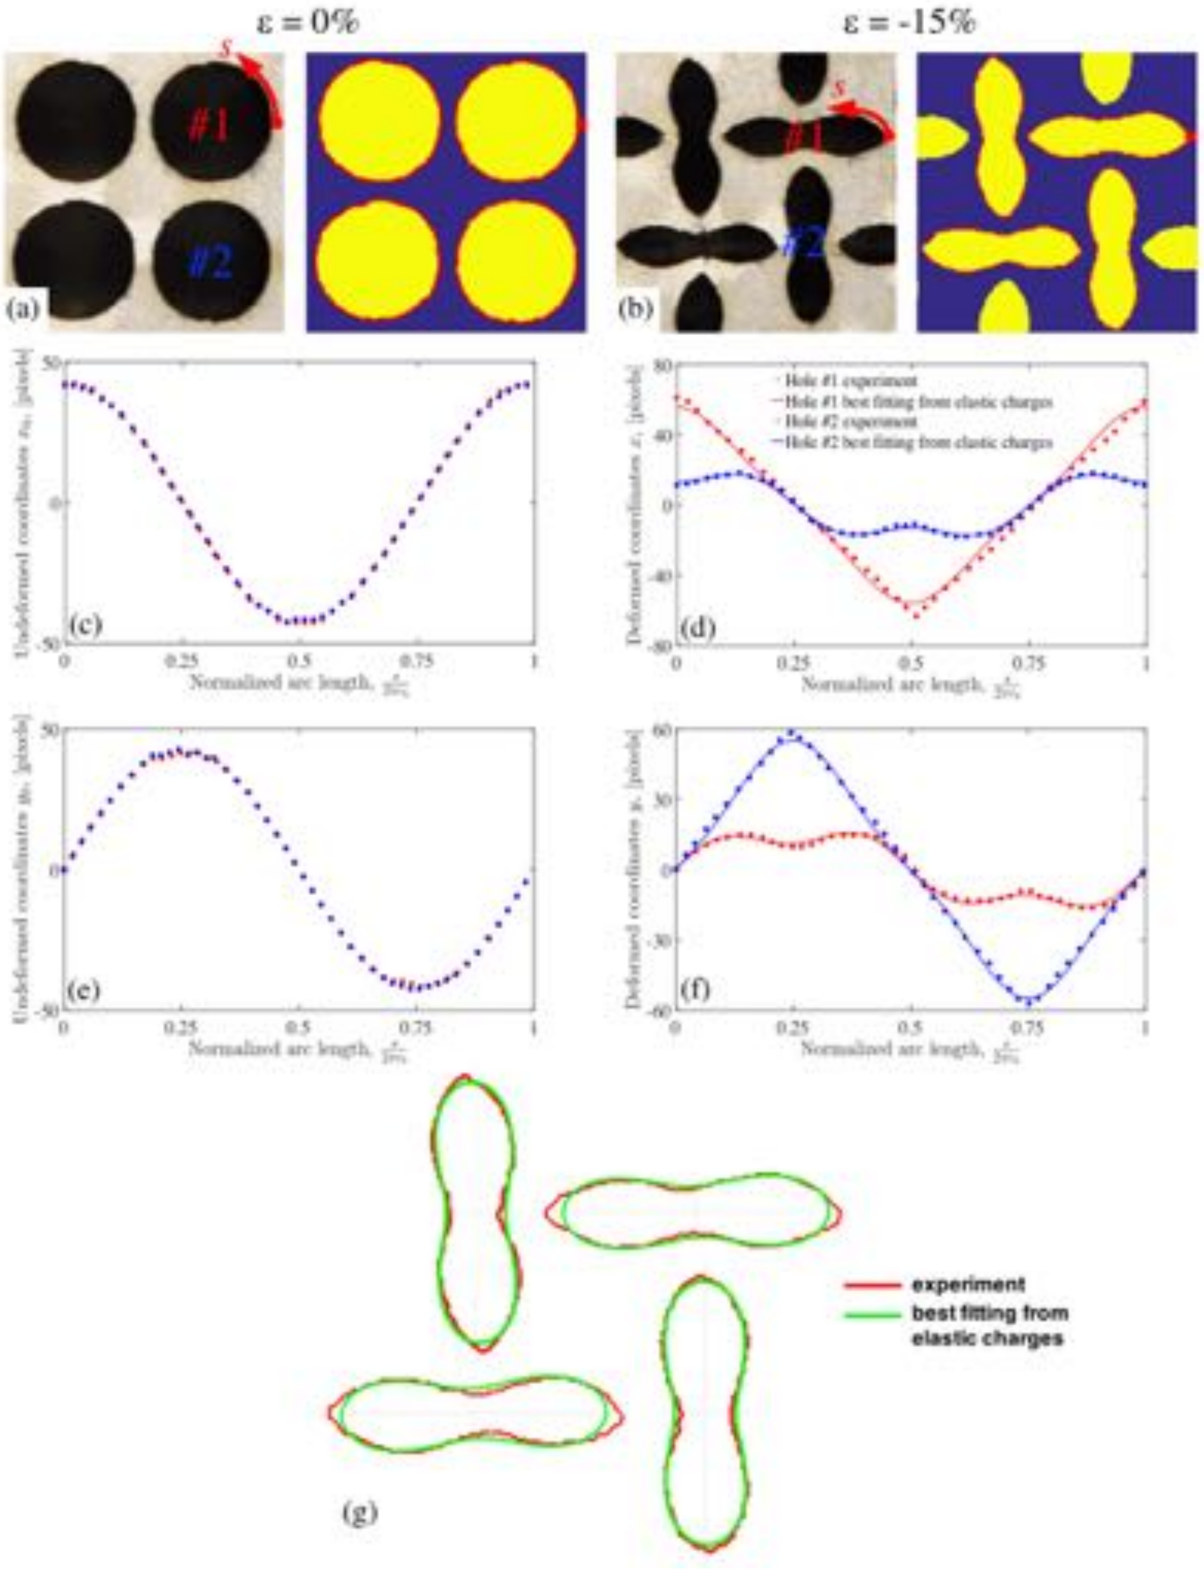


FIG. S2. **Fitting procedure.** (a)-(b) Snapshots of the four central holes of the samples and corresponding digitalized images at (a) $\varepsilon = 0$ and (b) $\varepsilon = -0.15$. (c) Coordinate $x_0$ as a function of the arch length $s$ for holes #1 and #2 at $\varepsilon = 0$. (d) Coordinate $x$ as a function of the arch length $s$ for holes #1 and #2 at $\varepsilon = -0.15$. Markers and lines corresponds to experimental data and the best fitting generated by the elastic charges, respectively. (e) Coordinate $y_0$ as a function of the arch length $s$ for holes #1 and #2 at $\varepsilon = 0$. (f) Coordinate $y$ as a function of the arch length $s$ for holes #1 and #2 at $\varepsilon = -0.15$. Markers and lines corresponds to experimental data and the best fitting generated by the elastic charges, respectively. (g) Experimentally observed hole boundaries (red lines) and best fitting generated by the elastic charges at $\varepsilon = -0.15$.

## ADDITIONAL EXPERIMENTAL RESULTS

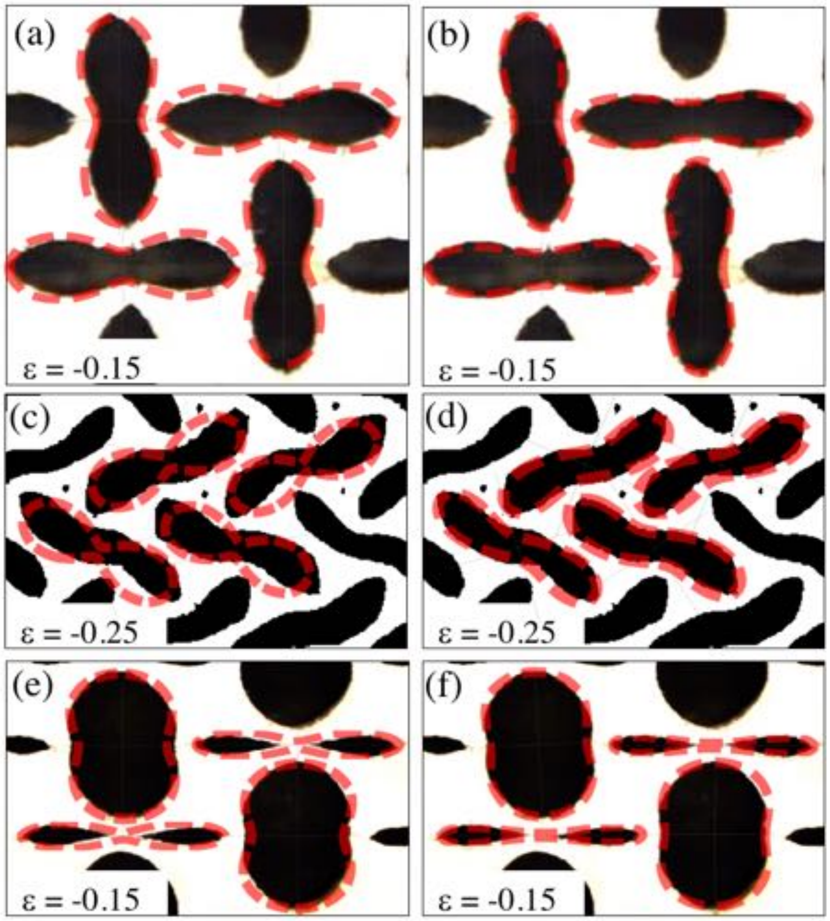


FIG. S3. **Effect of quadrupole and hexadecapole charges.** (a)-(b) Experimental images of the four central holes of Sample#1 at $\varepsilon = -0.15$ and best-fitting hole shapes generated by the elastic charges (dashed lines) when (a) the contribution of the hexadecapoles is neglected and (b) is considered. (c)-(d) Experimental images of the four central holes of Sample#2 at $\varepsilon = -0.25$ and best-fitting hole shapes generated by the elastic charges (dashed lines) when (a) the contribution of the hexadecapoles is neglected and (b) is considered.(e)-(f) Experimental images of the four central holes of Sample#3 at $\varepsilon = -0.15$ and best-fitting hole shapes generated by the elastic charges (dashed lines) when (a) the contribution of the hexadecapoles is neglected and (b) is considered.

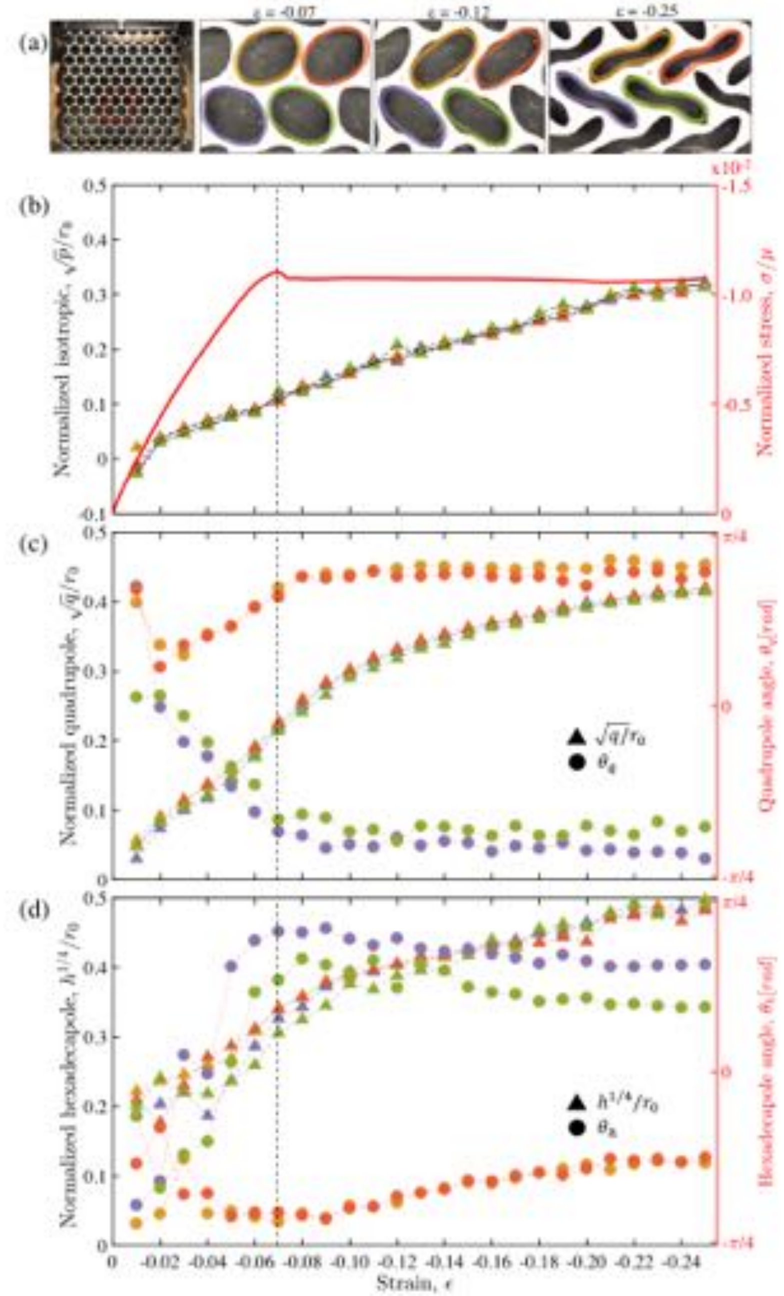


FIG. S4. **Response under uniaxial compression applied in vertical direction for a mechanical metamaterial comprising a triangular array of circular holes.** (a) Experimental images of the four central holes at different levels of applied strain. The colored lines represent the best-fitting hole shapes generated with the elastic charges. (b) Evolution of the normalized isotropic charges as a function of the applied strain for the four central holes (triangular markers - left axis); stress-strain curve (red line - right axis). (c) Evolution of the normalized magnitude (triangular markers - left axis) and orientation (circular markers - right axis) of the quadrupole charges as a function of the applied strain for the four central holes. (d) Evolution of the normalized magnitude (triangular markers - left axis) and orientation (circular markers - right axis) of the hexadecapole charges as a function of the applied strain for the four central holes.

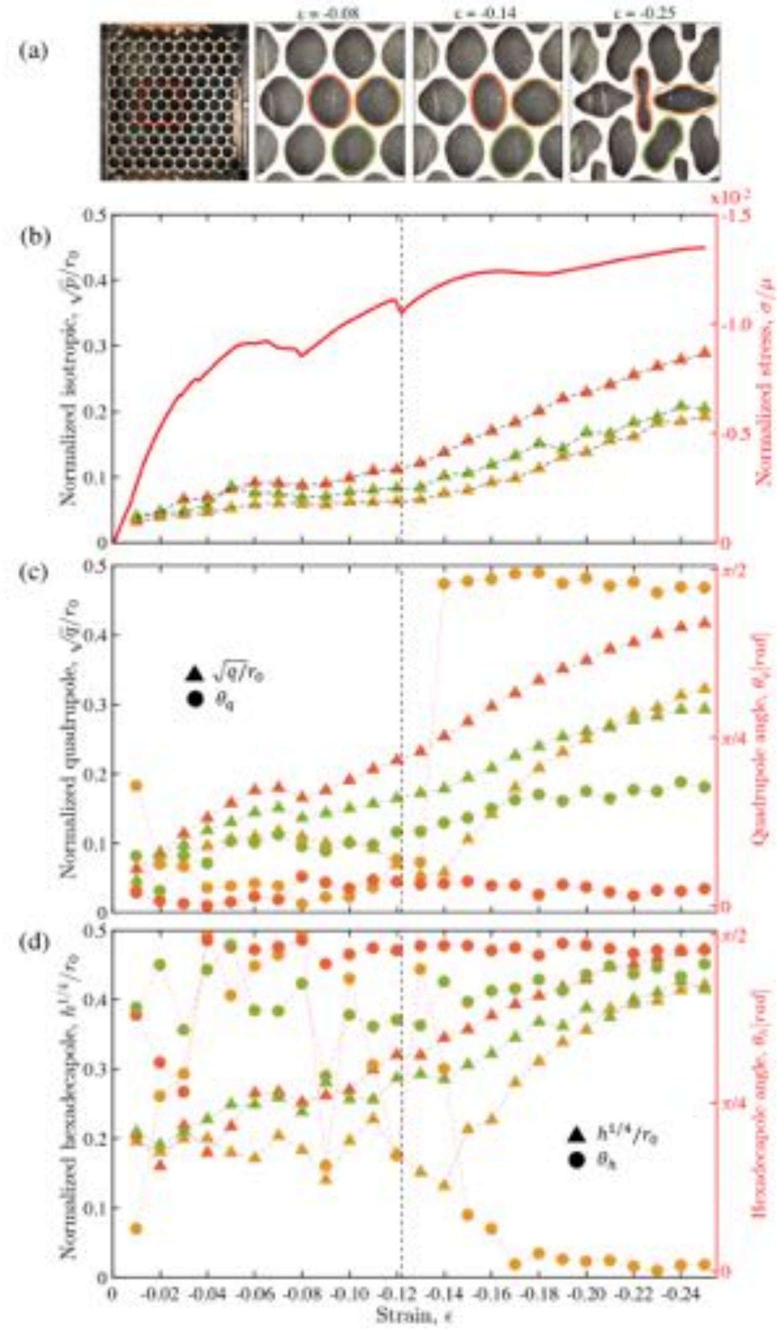


FIG. S5. **Response under uniaxial compression applied in horizontal direction for a mechanical metamaterial comprising a triangular array of circular holes.** (a) Experimental images of the four central holes at different levels of applied strain. The colored lines represent the best-fitting hole shapes generated with the elastic charges.(b) Evolution of the normalized isotropic charges as a function of the applied strain for the four central holes (triangular markers - left axis); stress-strain curve (red line - right axis). (c) Evolution of the normalized magnitude (triangular markers - left axis) and orientation (circular markers - right axis) of the quadrupole charges as a function of the applied strain for the four central holes. (d) Evolution of the normalized magnitude (triangular markers - left axis) and orientation (circular markers - right axis) of the hexadecapole charges as a function of the applied strain for the four central holes.

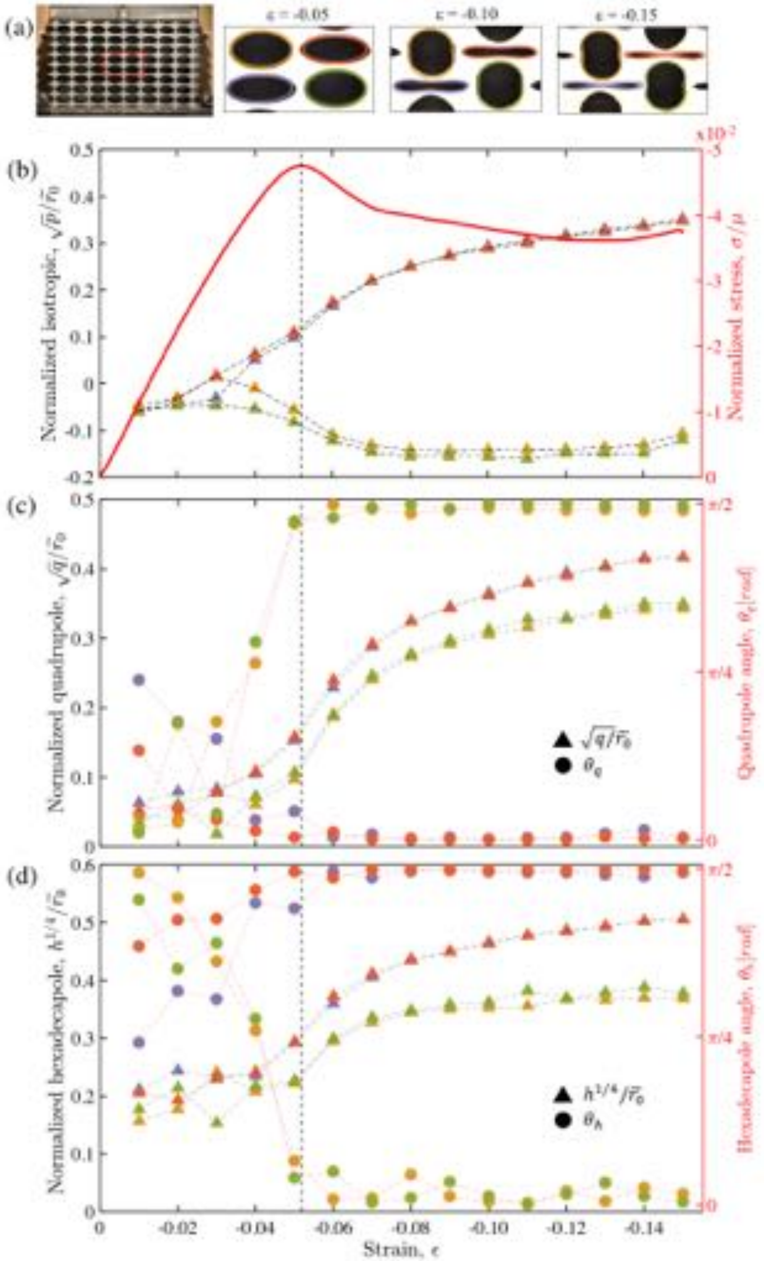


FIG. S6. **Response under uniaxial compression applied in vertical direction for a mechanical metamaterial comprising a rectangular array of elliptical holes.** (a) Experimental images of the four central holes at different levels of applied strain. The colored lines represent the best-fitting hole shapes generated with the elastic charges. (b) Evolution of the normalized isotropic charges as a function of the applied strain for the four central holes (triangular markers - left axis); stress-strain curve (red line - right axis). (c) Evolution of the normalized magnitude (triangular markers - left axis) and orientation (circular markers - right axis) of the quadrupole charges as a function of the applied strain for the four central holes. (d) Evolution of the normalized magnitude (triangular markers - left axis) and orientation (circular markers - right axis) of the hexadecapole charges as a function of the applied strain for the four central holes.Note that for this sample all charge magnitudes are normalized by $\widetilde{r_0} = (a + b)/2$, where $a$ and $b$ denote the major and minor semi-axes of the ellipses, respectively.
